# Supplementary material for: Error estimates for solid-state density-functional theory predictions: an overview by means of the ground-state elemental crystals
Source: arXiv:1204.2733 ancillary file (2013-08-05)
Supplement: Supplementary file 1 [file SupplMat.pdf]

# Error estimates for solid-state density-functional theory predictions: an overview by means of the ground-state elemental crystals

K. Lejaeghere, V. Van Speybroeck, G. Van Oost, and S. Cottenier
Critical Reviews in Solid State and Materials Sciences (2014)
Supplementary Material

All citations in this document refer to the list that is given in the end, and not to the bibliography of the main paper.

## 1. Computational parameters

In the main article three DFT codes are evaluated. The current section lists the most important settings, applied to all test set compounds.

**VASP**

*cut-off energy*

400 eV for most elements
600 eV for He, B, C, N, O, F, and Ne

*self-consistent cycle*

$10^{-4}$ eV energy convergence criterion

*reciprocal space representation*

6750 / N k-points for N-atom cells

*FFT grid*

default (2 $G_{cut}$ x 2 $G_{cut}$ x 2 $G_{cut}$ ; $G_{cut}$ being the cut-off electronic wave vector)

*augmentation charge grid*

default (4 $G_{cut}$ x 4 $G_{cut}$ x 4 $G_{cut}$)

*potential files*

see Tab. 1.1

**WIEN2k**

*muffin tin radius*

2.30 a.u. when this does not cause the atomic spheres to overlap
else: all but touching spheres in a cell with volume $V_0$ - 6%

*spherical harmonic truncation*

lmax = 14 inside the muffin-tin spheres
lmax = 6 for matrix elements with contributions outside of the muffin-tin sphere

*core-valence separation*

see Tab. 1.2

*product of the muffin tin radius and the maximum wave vector*

see Tab. 1.2

*Fourier expansion truncation*

$G_{max}$ equal to approximately 3 $G_{min}$

*FFT mesh parameters*

automatically calculated, by means of a multiplicative factor of 4

*reciprocal space representation*

30 000 k points per unit cell volume of 120 a.u. (full Brillouin zone)

*energy level broadening*

Fermi-Dirac distribution corresponding to $k_B$ T = 0.001 Ry

*self-consistent cycle*

$5 \cdot 10^{-7}$ *e* charge convergence criterion

**GPAW**

*grid spacing*

0.075 Å

*reciprocal space representation*

6750 / N k-points for N-atom cells

*self-consistent cycle*

0.5 meV per valence electron energy convergence criterion

$1 \cdot 10^{-4}$ *e* per valence electron charge convergence criterion

*energy level broadening*

Fermi-Dirac distribution corresponding to $k_B$ T = 0.1 eV

**Tab. 1.1** VASP potentials used for the elemental crystals

| | potential file |
|---|---|
| H | PAW_PBE H 15Jun2001 |
| He | PAW_PBE He 05Jan2001 |
| Li | PAW_PBE Li_sv 23Jan2001 |
| Be | PAW_PBE Be 06Sep2000 |
| B | PAW_PBE B 06Sep2000 |
| C | PAW_PBE C 08Apr2002 |
| N | PAW_PBE N 08Apr2002 |
| O | PAW_PBE O 08Apr2002 |
| F | PAW_PBE F 08Apr2002 |
| Ne | PAW_PBE Ne 05Jan2001 |
| Na | PAW_PBE Na_pv 05Jan2001 |
| Mg | PAW_PBE Mg 05Jan2001 |
| Al | PAW_PBE Al 04Jan2001 |
| Si | PAW_PBE Si 05Jan2001 |
| P | PAW_PBE P 17Jan2003 |
| S | PAW_PBE S 17Jan2003 |
| Cl | PAW_PBE Cl 17Jan2003 |
| Ar | PAW_PBE Ar 07Sep2000 |
| K | PAW_PBE K_sv 06Sep2000 |
| Ca | PAW_PBE Ca_pv 06Sep2000 |
| Sc | PAW_PBE Sc_sv 07Sep2000 |
| Ti | PAW_PBE Ti_pv 07Sep2000 |
| V | PAW_PBE V_pv 07Sep2000 |
| Cr | PAW_PBE Cr_pv 07Sep2000 |
| Mn | PAW_PBE Mn_pv 07Sep2000 |
| Fe | PAW_PBE Fe 06Sep2000 |
| Co | PAW_PBE Co 06Sep2000 |
| Ni | PAW_PBE Ni 06Sep2000 |
| Cu | PAW_PBE Cu 05Jan2001 |
| Zn | PAW_PBE Zn 06Sep2000 |
| Ga | PAW_PBE Ga_d 06Sep2000 |
| Ge | PAW_PBE Ge_d 06Sep2000 |
| As | PAW_PBE As 06Sep2000 |
| Se | PAW_PBE Se 06Sep2000 |
| Br | PAW_PBE Br 06Sep2000 |
| Kr | PAW_PBE Kr 07Sep2000 |
| Rb | PAW_PBE Rb_sv 06Sep2000 |
| Sr | PAW_PBE Sr_sv 07Sep2000 |
| Y | PAW_PBE Y_sv 06Sep2000 |
| Zr | PAW_PBE Zr_sv 07Sep2000 |
| Nb | PAW_PBE Nb_pv 08Apr2002 |
| Mo | PAW_PBE Mo_pv 08Apr2002 |
| Tc | PAW_PBE Tc_pv 06Sep2000 |
| Ru | PAW_PBE Ru 06Sep2000 |
| Rh | PAW_PBE Rh 06Sep2000 |
| Pd | PAW_PBE Pd 05Jan2001 |
| Ag | PAW_PBE Ag 06Sep2000 |

| | |
|---|---|
| Cd | PAW_PBE Cd 06Sep2000 |
| In | PAW_PBE In_d 06Sep2000 |
| Sn | PAW_PBE Sn_d 06Sep2000 |
| Sb | PAW_PBE Sb 06Sep2000 |
| Te | PAW_PBE Te 08Apr2002 |
| I | PAW_PBE I 08Apr2002 |
| Xe | PAW_PBE Xe 07Sep2000 |
| Cs | PAW_PBE Cs_sv 08Apr2002 |
| Ba | PAW_PBE Ba_sv 06Sep2000 |
| Lu | PAW_PBE Lu_3 06Sep2000 |
| Hf | PAW_PBE Hf_pv 06Sep2000 |
| Ta | PAW_PBE Ta_pv 07Sep2000 |
| W | PAW_PBE W_pv 06Sep2000 |
| Re | PAW_PBE Re 17Jan2003 |
| Os | PAW_PBE Os_pv 20Jan2003 |
| Ir | PAW_PBE Ir 06Sep2000 |
| Pt | PAW_PBE Pt 05Jan2001 |
| Au | PAW_PBE Au 06Sep2000 |
| Hg | PAW_PBE Hg 06Sep2000 |
| Tl | PAW_PBE Tl_d 06Sep2000 |
| Pb | PAW_PBE Pb_d 06Sep2000 |
| Bi | PAW_PBE Bi_d 06Sep2000 |
| Po | PAW_PBE Po_d 25May2007 |
| Rn | PAW_PBE Rn 28Aug2006 |

**Tab. 1.2** WIEN2k core-valence separation and $RK_{max}$ used for the elemental crystals

| | highest core | lowest valence | $RK_{max}$ |
|---|---|---|---|
| H | | 1s | 5.0 |
| He | | 1s | 10.0 |
| Li | | 1s | 10.0 |
| Be | | 1s | 10.0 |
| B | 1s | 2s | 7.5 |
| C | 1s | 2s | 7.5 |
| N | 1s | 2s | 7.5 |
| O | 1s | 2s | 7.5 |
| F | 1s | 2s | 8.0 |
| Ne | 1s | 2s | 10.0 |
| Na | 1s | 2s | 10.0 |
| Mg | 1s | 2s | 10.0 |
| Al | 2s | 2p | 10.0 |
| Si | 2s | 2p | 10.0 |
| P | 2s | 2p | 9.0 |
| S | 2p | 3s | 10.0 |
| Cl | 2p | 3s | 8.0 |
| Ar | 2p | 3s | 10.0 |
| K | 2p | 3s | 10.0 |
| Ca | 2p | 3s | 10.0 |
| Sc | 2p | 3s | 10.0 |
| Ti | 2p | 3s | 10.0 |
| V | 2p | 3s | 10.0 |
| Cr | 2p | 3s | 10.0 |
| Mn | 2p | 3s | 10.0 |
| Fe | 2p | 3s | 10.0 |
| Co | 2p | 3s | 10.0 |
| Ni | 2p | 3s | 10.0 |
| Cu | 2p | 3s | 10.0 |
| Zn | 2p | 3s | 10.0 |
| Ga | 3p | 3d | 10.0 |
| Ge | 3p | 3d | 10.0 |
| As | 3p | 3d | 10.0 |
| Se | 3p | 3d | 10.0 |
| Br | 3p | 3d | 10.0 |
| Kr | 3p | 3d | 10.0 |
| Rb | 3d | 4s | 10.0 |
| Sr | 3d | 4s | 10.0 |
| Y | 3d | 4s | 10.0 |
| Zr | 3d | 4s | 10.0 |
| Nb | 3d | 4s | 10.0 |
| Mo | 3d | 4s | 10.0 |
| Tc | 3d | 4s | 10.0 |
| Ru | 3d | 4s | 10.0 |
| Rh | 3d | 4s | 10.0 |
| Pd | 3d | 4s | 10.0 |
| Ag | 3d | 4s | 10.0 |

| | | | |
|---|---|---|---|
| Cd | 3d | 4s | 10.0 |
| In | 4s | 4p | 10.0 |
| Sn | 4s | 4p | 10.0 |
| Sb | 4s | 4p | 10.0 |
| Te | 4s | 4p | 10.0 |
| I | 4s | 4p | 10.0 |
| Xe | 4s | 4p | 10.0 |
| Cs | 4p | 4d | 10.0 |
| Ba | 4p | 4d | 10.0 |
| Lu | 4d | 5s | 12.0 |
| Hf | 4d | 5s | 12.0 |
| Ta | 4d | 5s | 12.0 |
| W | 4d | 5s | 12.0 |
| Re | 4d | 5s | 12.0 |
| Os | 4d | 5s | 12.0 |
| Ir | 4d | 5s | 12.0 |
| Pt | 4d | 5s | 12.0 |
| Au | 4d | 5s | 12.0 |
| Hg | 4d | 5s | 12.0 |
| Tl | 4f | 5p | 12.0 |
| Pb | 4f | 5p | 12.0 |
| Bi | 4f | 5p | 12.0 |
| Po | 4f | 5p | 12.0 |
| Rn | 4f | 5p | 12.0 |

## 2. Difference with experiment

**Tab. 2.1** Cohesive energy (in kJ/mol) by means of VASP-PBE and from experiment, with ($\Delta E_{coh,exp}$) and without ($\Delta E_{coh,exp}^0$) correcting for the zero-point energy ζ , and the Debye temperature $\Theta_D$ (in K) necessary for the calculation of ζ

| | **$\Delta E_{coh,VASP}$** | **$\Delta E_{coh,exp}$** | **$\Delta E_{coh,exp}^0$** | **$\Theta_D$** | **ζ** |
|---|---|---|---|---|---|
| H | 219 | | | | |
| He | 1.10 | | | | |
| Li | 155 | 161 | 158 [1] | 344 [1] | 3.2 |
| Be | 360 | 333 | 320 [1] | 1440 [1] | 13.5 |
| B | 600 | 569 | 561 [1] | 805 [4] | 7.5 |
| C | 758 | 719 | 715 [2] | 402 [3] | 3.8 |
| N | 503 | 475 | 474 [1] | 70 [4] | 0.7 |
| O | 294 | 252 | 251 [1] | 93 [4] | 0.5 |
| F | 114 | 81 | 81 [1] | 65 [4] | 0.5 |
| Ne | 1.80 | 2.62 | 1.92 [1] | 75 [1] | 0.7 |
| Na | 104 | 108 | 107 [1] | 158 [1] | 1.5 |
| Mg | 145 | 149 | 145 [1] | 400 [1] | 3.7 |
| Al | 331 | 331 | 327 [1] | 428 [1] | 4.0 |
| Si | 439 | 452 | 446 [1] | 645 [1] | 6.0 |
| P | 336 | 333 | 331 [1] | 231 [4] | 2.2 |
| S | 294 | 277 | 275 [1] | 182 [4] | 1.7 |
| Cl | 141 | 137 | 135 [1] | 142 [4] | 2.0 |
| Ar | 9.16 | 8.60 | 7.74 [1] | 92 [1] | 0.9 |
| K | 83.9 | 91.0 | 90.1 [1] | 91 [1] | 0.9 |
| Ca | 185 | 180 | 178 [1] | 230 [1] | 2.2 |
| Sc | 400 | 379 | 376 [1] | 360 [1] | 3.4 |
| Ti | 528 | 472 | 468 [1] | 420 [1] | 3.9 |
| V | 571 | 516 | 512 [1] | 380 [1] | 3.6 |
| Cr | 390 | 401 | 395 [1] | 630 [1] | 5.9 |
| Mn | 372 | 286 | 282 [1] | 410 [1] | 3.8 |
| Fe | 468 | 417 | 413 [1] | 470 [1] | 4.4 |
| Co | 496 | 428 | 424 [1] | 445 [1] | 4.2 |
| Ni | 466 | 432 | 428 [1] | 450 [1] | 4.2 |
| Cu | 335 | 339 | 336 [1] | 343 [1] | 3.2 |
| Zn | 106 | 133 | 130 [1] | 327 [1] | 3.1 |
| Ga | 254 | 274 | 271 [1] | 320 [1] | 3.0 |
| Ge | 361 | 375 | 372 [1] | 374 [1] | 3.5 |
| As | 286 | 287.9 | 285.3 [1] | 282 [1] | 2.6 |
| Se | 251 | 238 | 237 [1] | 90 [1] | 0.8 |
| Br | 131 | 120 | 118 [1] | 104 [4] | 1.6 |
| Kr | 2.34 | 11.9 | 11.2 [1] | 72 [1] | 0.7 |
| Rb | 74.7 | 82.7 | 82.2 [1] | 56 [1] | 0.5 |
| Sr | 156 | 167 | 166 [1] | 147 [1] | 1.4 |
| Y | 402 | 425 | 422 [1] | 280 [1] | 2.6 |
| Zr | 604 | 606 | 603 [1] | 291 [1] | 2.7 |
| Nb | 669 | 733 | 730 [1] | 275 [1] | 2.6 |
| Mo | 603 | 662 | 658 [1] | 450 [1] | 4.2 |

| | | | | | |
|---|---|---|---|---|---|
| Tc | 658 | 665 | 661 [1] | 387 [4] | 3.6 |
| Ru | 644 | 656 | 650 [1] | 600 [1] | 5.6 |
| Rh | 567 | 558 | 554 [1] | 480 [1] | 4.5 |
| Pd | 357 | 379 | 376 [1] | 274 [1] | 2.6 |
| Ag | 240 | 286 | 284 [1] | 225 [1] | 2.1 |
| Cd | 71.5 | 114 | 112 [1] | 209 [1] | 2.0 |
| In | 223 | 244 | 243 [1] | 108 [1] | 1.0 |
| Sn | 306 | 305 | 303 [1] | 200 [1] | 1.9 |
| Sb | 261 | 267 | 265 [1] | 211 [1] | 2.0 |
| Te | 233 | 212 | 211 [1] | 153 [1] | 1.4 |
| I | 125 | 109 | 107 [1] | 87 [4] | 1.6 |
| Xe | 2.69 | 16.5 | 15.9 [1] | 64 [1] | 0.6 |
| Cs | 69.0 | 78.0 | 77.6 [1] | 38 [1] | 0.4 |
| Ba | 182 | 184 | 183 [1] | 110 [1] | 1.0 |
| Lu | 395 | 430 | 428 [1] | 210 [1] | 2.0 |
| Hf | 606 | 623 | 621 [1] | 252 [1] | 2.4 |
| Ta | 766 | 784 | 782 [1] | 240 [1] | 2.2 |
| W | 852 | 863 | 859 [1] | 400 [1] | 3.7 |
| Re | 760 | 779 | 775 [1] | 430 [1] | 4.0 |
| Os | 770 | 793 | 788 [1] | 500 [1] | 4.7 |
| Ir | 676 | 674 | 670 [1] | 420 [1] | 3.9 |
| Pt | 514 | 566 | 564 [1] | 240 [1] | 2.2 |
| Au | 300 | 370 | 368 [1] | 165 [1] | 1.5 |
| Hg | 20 | 66 | 65 [1] | 71.9 [1] | 0.7 |
| Tl | 146 | 183 | 182 [1] | 78.5 [1] | 0.7 |
| Pb | 189 | 197 | 196 [1] | 105 [1] | 1.0 |
| Bi | 200 | 211 | 210 [1] | 119 [1] | 1.1 |
| Po | 157 | 145 | 144 [1] | 92 [4] | 0.9 |
| Rn | 3.78 | 19.6 | 19.5 [1] | 15 [4] | 0.1 |

**Tab. 2.2** Equilibrium volume (in $Å^3$/atom) by means of VASP-PBE and from experiment, with ($V_{0,exp}$) and without ($V_{0,exp}^0$) thermally correcting for $\Delta V^{(1)}$ and $\Delta V^{(2)}$ (see article), and the thermal volume expansion coefficient at room temperature $\alpha_{V,rt}$ (in $10^{-5}$/K) necessary for the calculation of $\Delta V^{(1)}$

| | $V_{0,VASP}$ | $V_{0,exp}$ | $V_{0,exp}^0$ | $\Delta V^{(1)}$ | $\Delta V^{(2)}$ | $\alpha_{V,rt}$ |
|---|---|---|---|---|---|---|
| H | 17.41 | 6.58 | 19.03 [5] | | 12.45 | |
| He | 17.73 | 9.40 | 31.7 [5] | | 22.33 | |
| Li | 20.28 | 20.41 | 20.99 [5] | | 0.58 | 13.8 [14] |
| Be | 7.92 | 7.82 | 8.11 [5] | 0.04 | 0.25 | 3.39 [14] |
| B | 7.25 | 7.16 | 7.29 [5] | 0.03 | 0.11 | 2.49 [14] |
| C | 11.66 | 8.06 | 8.82 [5] | 0.03 | 0.73 | 2.4 [15] |
| N | 29.65 | 21.09 | 22.47 [6] | | 1.39 | |
| O | 19.18 | 15.98 | 17.36 [5] | | 1.38 | |
| F | 19.52 | 14.47 | 16.05 [7] | | 1.58 | |
| Ne | 24.69 | 17.85 | 22.2 [8] | | 4.35 | |
| Na | 37.07 | 37.18 | 37.74 [5] | | 0.56 | 21.3 [14] |
| Mg | 22.85 | 22.65 | 23.24 [5] | 0.26 | 0.33 | 7.44 [14] |
| Al | 16.49 | 16.27 | 16.6 [5] | 0.17 | 0.16 | 6.93 [14] |
| Si | 20.45 | 19.82 | 20.02 [5] | 0.02 | 0.17 | 0.78 [14] |
| P | 21.38 | 18.50 | 18.99 [5] | 0.28 | 0.21 | 9.9 [16] |
| S | 38.48 | 24.63 | 25.52 [5] | 0.43 | 0.46 | 11.19 [17] |
| Cl | 38.18 | 26.95 | 27.53 [9] | | 0.58 | |
| Ar | 52.67 | 35.55 | 37.2 [10] | | 1.65 | |
| K | 73.85 | 72.20 | 75.72 [5] | 2.84 | 0.68 | 24.99 [14] |
| Ca | 42.17 | 42.95 | 43.63 [5] | 0.44 | 0.25 | 6.69 [14] |
| Sc | 24.66 | 24.77 | 25 [5] | 0.11 | 0.12 | 3.06 [14] |
| Ti | 17.37 | 17.50 | 17.64 [5] | 0.07 | 0.07 | 2.58 [14] |
| V | 13.49 | 13.81 | 13.92 [5] | 0.05 | 0.06 | 2.52 [14] |
| Cr | 11.83 | 11.82 | 12 [5] | 0.03 | 0.15 | 1.47 [14] |
| Mn | 11.10 | 11.97 | 12.2 [5] | 0.12 | 0.11 | 6.51 [14] |
| Fe | 11.37 | 11.64 | 11.78 [5] | 0.06 | 0.08 | 3.54 [14] |
| Co | 10.88 | 10.96 | 11.08 [5] | 0.06 | 0.06 | 3.9 [14] |
| Ni | 10.94 | 10.81 | 10.93 [5] | 0.07 | 0.06 | 4.02 [14] |
| Cu | 12.03 | 11.65 | 11.81 [5] | 0.09 | 0.08 | 4.95 [14] |
| Zn | 15.35 | 14.86 | 15.21 [5] | 0.21 | 0.14 | 9.06 [14] |
| Ga | 20.36 | 19.15 | 19.47 [5] | 0.16 | 0.16 | 5.4 [14] |
| Ge | 23.91 | 22.44 | 22.64 [5] | 0.06 | 0.14 | 1.74 [14] |
| As | 22.73 | 21.23 | 21.52 [5] | 0.16 | 0.13 | 5.04 [18] |
| Se | 29.84 | 26.22 | 27.27 [5] | 0.68 | 0.37 | 16.61 [14] |
| Br | 39.29 | 31.47 | 31.89 [9] | | 0.42 | |
| Kr | 66.44 | 44.04 | 45 [11] | | 0.96 | |
| Rb | 91.24 | 89.16 | 92.84 [5] | 3.28 | 0.40 | 23.55 [19] |
| Sr | 54.53 | 55.60 | 56.32 [5] | 0.57 | 0.15 | 6.75 [14] |
| Y | 32.92 | 32.95 | 33.18 [5] | 0.16 | 0.07 | 3.18 [14] |
| Zr | 23.53 | 23.18 | 23.28 [5] | 0.06 | 0.04 | 1.71 [14] |
| Nb | 18.34 | 17.97 | 18.07 [5] | 0.06 | 0.04 | 2.19 [14] |
| Mo | 15.92 | 15.51 | 15.58 [5] | 0.03 | 0.04 | 1.44 [14] |
| Tc | 14.60 | 14.22 | 14.3 [5] | 0.05 | 0.04 | 2.1 [1,20] |

| | | | | | | |
|---|---|---|---|---|---|---|
| Ru | 13.84 | 13.45 | 13.57 [5] | 0.04 | 0.08 | 1.92 [14] |
| Rh | 14.18 | 13.57 | 13.67 [5] | 0.05 | 0.05 | 2.46 [14] |
| Pd | 15.44 | 14.56 | 14.69 [5] | 0.08 | 0.05 | 3.54 [14] |
| Ag | 18.05 | 16.85 | 17.06 [5] | 0.15 | 0.06 | 5.67 [14] |
| Cd | 23.05 | 21.01 | 21.44 [5] | 0.30 | 0.14 | 9.24 [14] |
| In | 27.54 | 25.70 | 26.17 [5] | 0.38 | 0.09 | 9.63 [14] |
| Sn | 36.86 | 33.97 | 34.16 [5] | 0.08 | 0.11 | 1.62 [14] |
| Sb | 31.79 | 29.68 | 29.97 [5] | 0.15 | 0.14 | 3.3 [14] |
| Te | 34.98 | 33.30 | 33.94 [5] | 0.26 | 0.38 | 5.04 [14] |
| I | 49.78 | 37.04 | 42.63 [5] | 5.10 | 0.49 | 79.7 [20] |
| Xe | 87.78 | 56.87 | 57.6 [12] | | 0.73 | |
| Cs | 116.96 | 110.32 | 115.79 [5] | 5.05 | 0.41 | 29.1 [14] |
| Ba | 63.55 | 62.29 | 62.99 [5] | 0.58 | 0.12 | 6.18 [14] |
| Lu | 29.32 | 29.27 | 29.5 [5] | 0.13 | 0.10 | 2.97 [14] |
| Hf | 22.42 | 22.30 | 22.41 [5] | 0.06 | 0.05 | 1.77 [14] |
| Ta | 18.30 | 17.93 | 18.01 [5] | 0.05 | 0.03 | 1.89 [14] |
| W | 16.28 | 15.80 | 15.86 [5] | 0.03 | 0.03 | 1.35 [14] |
| Re | 14.96 | 14.62 | 14.7 [5] | 0.04 | 0.04 | 1.86 [14] |
| Os | 14.44 | 13.85 | 13.91 [5] | 0.03 | 0.03 | 1.53 [14] |
| Ir | 14.61 | 14.06 | 14.14 [5] | 0.04 | 0.04 | 1.92 [14] |
| Pt | 15.78 | 15.02 | 15.11 [5] | 0.06 | 0.03 | 2.64 [14] |
| Au | 18.05 | 16.82 | 16.97 [5] | 0.11 | 0.04 | 4.26 [14] |
| Hg | 28.27 | 22.25 | 22.55 [13] | | 0.30 | |
| Tl | 31.17 | 27.99 | 28.41 [5] | 0.38 | 0.03 | 8.97 [14] |
| Pb | 32.27 | 29.86 | 30.34 [5] | 0.39 | 0.08 | 8.67 [14] |
| Bi | 38.27 | 35.13 | 35.38 [5] | 0.21 | 0.04 | 4.02 [14] |
| Po | 39.62 | 36.93 | 37.43 [5] | 0.40 | 0.10 | 7.05 [14] |
| Rn | 89.60 | | | | | |

**Tab. 2.3** Bulk modulus (in GPa) by means of VASP-PBE and from experiment, with ($B_{0,exp}$) and without ($B_{0,exp}^{0}$) thermally correcting for $\Delta B^{(1)}$ and $\Delta B^{(2)}$ (see article)

| | $B_{0,VASP}$ | $B_{0,exp}$ | $B_{0,exp}^{0}$ | $\Delta B^{(1)}$ | $\Delta B^{(2)}$ |
|---|---|---|---|---|---|
| H | 0.4 | 0.5 | 0.2 [1] | | -0.27 |
| He | 0.9 | 0.42 | 0.08 [1] | | -0.34 |
| Li | 13.8 | 13.1 | 11.6 [1] | -0.84 | -0.62 |
| Be | 122.8 | 108.1 | 100.3 [1] | -1.65 | -6.20 |
| B | 210.5 | 185.9 | 178 [1] | -2.65 | -5.27 |
| C | 1.6 | 55.6 | 33.8 [21] | -1.08 | -20.71 |
| N | 0.8 | 2.69 | 2.16 [22] | | -0.53 |
| O | 1.4 | | | | |
| F | 1.6 | | | | |
| Ne | 1.1 | 2.8 | 1.1 [23] | | -1.70 |
| Na | 7.7 | 7.9 | 6.8 [1] | -0.90 | -0.22 |
| Mg | 36.5 | 38.6 | 35.4 [1] | -1.90 | -1.31 |
| Al | 77.3 | 77.1 | 72.2 [1] | -3.34 | -1.60 |
| Si | 88.8 | 101.3 | 98.8 [1] | -0.51 | -1.97 |
| P | 7.3 | 33.2 | 30.4 [1] | -2.03 | -0.77 |
| S | 0.4 | 21.3 | 17.8 [1] | -2.02 | -1.48 |
| Cl | 1.3 | 40.8 | 11.7 [24] | -28.37 | -0.73 |
| Ar | 0.8 | 3.30 | 2.68 [25] | | -0.62 |
| K | 3.6 | 3.8 | 3.2 [1] | -0.49 | -0.06 |
| Ca | 17.5 | 15.9 | 15.2 [1] | -0.47 | -0.18 |
| Sc | 54.3 | 44.5 | 43.5 [1] | -0.56 | -0.48 |
| Ti | 112.5 | 107.4 | 105.1 [1] | -1.38 | -0.87 |
| V | 181.4 | 165.8 | 161.9 [1] | -2.53 | -1.41 |
| Cr | 177.0 | 204.6 | 190.1 [1] | -2.89 | -11.57 |
| Mn | 212.3 | 174.7 | 158 [26] | -10.18 | -6.52 |
| Fe | 185.9 | 175.1 | 168.3 [1] | -4.11 | -2.70 |
| Co | 208.4 | 198.4 | 191.4 [1] | -4.77 | -2.23 |
| Ni | 193.7 | 192.5 | 186 [1] | -4.49 | -1.97 |
| Cu | 136.7 | 144.3 | 137 [1] | -4.96 | -2.31 |
| Zn | 57.9 | 64.7 | 59.8 [1] | -3.58 | -1.29 |
| Ga | 48.3 | 60.2 | 56.9 [1] | -2.15 | -1.15 |
| Ge | 58.8 | 79.4 | 77.2 [1] | -0.96 | -1.23 |
| As | 25.5 | 40.8 | 39.4 [1] | -0.98 | -0.46 |
| Se | 4.4 | 10.9 | 9.1 [1] | -1.31 | -0.44 |
| Br | 1.6 | 25.6 | 13.3 [24] | -11.80 | -0.51 |
| Kr | 0.7 | 4.01 | 3.61 [27] | | -0.40 |
| Rb | 2.8 | 3.6 | 3.1 [1] | -0.43 | -0.03 |
| Sr | 11.1 | 12.0 | 11.6 [1] | -0.29 | -0.09 |
| Y | 41.4 | 37.3 | 36.6 [1] | -0.38 | -0.33 |
| Zr | 93.5 | 84.3 | 83.3 [1] | -0.55 | -0.43 |
| Nb | 171.7 | 173.2 | 170.2 [1] | -2.24 | -0.73 |
| Mo | 262.9 | 276.2 | 272.5 [1] | -2.34 | -1.37 |
| Tc | 298.4 | 303.1 | 297 [1] | -4.28 | -1.78 |
| Ru | 310.9 | 335.5 | 320.8 [1] | -6.11 | -8.61 |
| Rh | 254.3 | 277.1 | 270.4 [1] | -4.49 | -2.24 |

| | | | | | |
|---|---|---|---|---|---|
| Pd | 168.4 | 187.2 | 180.8 [1] | -4.80 | -1.59 |
| Ag | 89.3 | 105.7 | 100.7 [1] | -4.05 | -0.96 |
| Cd | 36.7 | 50.7 | 46.7 [1] | -3.17 | -0.79 |
| In | 35.7 | 44.7 | 41.1 [1] | -3.18 | -0.43 |
| Sn | 35.8 | 42.8 | 42.5 [28] | -0.04 | -0.28 |
| Sb | 30.7 | 39.5 | 38.3 [1] | -0.82 | -0.40 |
| Te | 17.8 | 26.2 | 23 [1] | -1.46 | -1.75 |
| I | 1.9 | 23.9 | 13.6 [24] | -9.76 | -0.59 |
| Xe | 0.5 | 3.83 | 3.64 [29] | | -0.19 |
| Cs | 2.0 | 2.3 | 2 [1] | -0.33 | -0.01 |
| Ba | 8.9 | 10.6 | 10.3 [1] | -0.23 | -0.06 |
| Lu | 47.3 | 42.0 | 41.1 [1] | -0.64 | -0.27 |
| Hf | 107.2 | 110.7 | 109 [1] | -1.14 | -0.52 |
| Ta | 193.0 | 202.7 | 200 [1] | -2.13 | -0.56 |
| W | 298.0 | 327.5 | 323.2 [1] | -2.83 | -1.45 |
| Re | 366.4 | 380.8 | 372 [1] | -5.61 | -3.15 |
| Os | 386.7 | 424.6 | 418 [1] | -4.32 | -2.29 |
| Ir | 337.0 | 362.2 | 355 [1] | -4.94 | -2.30 |
| Pt | 241.7 | 285.5 | 278.3 [1] | -5.71 | -1.50 |
| Au | 141.3 | 182.0 | 173.2 [1] | -7.08 | -1.72 |
| Hg | 12.9 | | | | |
| Tl | 26.7 | 37.4 | 35.9 [1] | -1.45 | -0.09 |
| Pb | 36.2 | 46.3 | 43 [1] | -2.98 | -0.36 |
| Bi | 22.5 | 32.1 | 31.5 [1] | -0.46 | -0.12 |
| Po | 33.9 | 27.4 | 26 [1] | -1.28 | -0.17 |
| Rn | 0.6 | | | | |

**Tab. 2.4** Pressure derivative of the bulk modulus $B_1$ (dimensionless) by means of VASP-PBE and from experiment

| | $B_{1,VASP}$ | $B_{1,exp}$ |
|---|---|---|
| H | 3.94 | |
| He | 7.52 | |
| Li | 3.16 | 3.51 [30] |
| Be | 3.24 | |
| B | 3.99 | |
| C | 9.89 | 8.9 [30] |
| N | 6.17 | |
| O | 5.62 | |
| F | 7.14 | |
| Ne | 8.13 | 9.23 [30] |
| Na | 3.27 | 4.13 [30] |
| Mg | 3.92 | 4.8 [30] |
| Al | 4.62 | 4.45 [30] |
| Si | 4.29 | 4.43 [30] |
| P | 13.56 | 4.5 [30] |
| S | 20.11 | 6.75 [30] |
| Cl | 11.01 | 5.2 [30] |
| Ar | 6.81 | 7.2 [30] |
| K | 3.70 | 4.089 [30] |
| Ca | 3.22 | 3.1 [30] |
| Sc | 3.41 | 2.8 [31] |
| Ti | 3.60 | 3.4 [30] |
| V | 3.81 | 4.135 [30] |
| Cr | 7.40 | 6.895 [30] |
| Mn | 6.40 | 6.6 [30] |
| Fe | 4.93 | 4.6 [30] |
| Co | 4.58 | 4.26 [32] |
| Ni | 4.97 | 4 [30] |
| Cu | 5.05 | 4.88 [30] |
| Zn | 5.77 | 4.4 [30] |
| Ga | 4.66 | |
| Ge | 4.85 | 4.76 [33] |
| As | 12.58 | 3.3 [34] |
| Se | 9.54 | 5.8 [30] |
| Br | 16.58 | 5.2 [30] |
| Kr | 8.49 | 7.2 [30] |
| Rb | 3.73 | 3.885 [30] |
| Sr | 5.02 | 2.485 [30] |
| Y | 3.21 | 2.2 [30] |
| Zr | 3.55 | 2.575 [30] |
| Nb | 3.99 | 4.015 [30] |
| Mo | 4.34 | 3.98 [30] |
| Tc | 4.55 | |
| Ru | 4.96 | 6.61 [32] |
| Rh | 5.24 | 4.5 [32] |

| | | |
|---|---|---|
| Pd | 5.54 | 5 [30] |
| Ag | 5.89 | 4.725 [30] |
| Cd | 6.21 | 4.9 [30] |
| In | 5.69 | 5.35 [30] |
| Sn | 4.83 | 4 [30] |
| Sb | 7.70 | 4.3 [30] |
| Te | 10.28 | 8.4 [30] |
| I | 13.57 | 6 [30] |
| Xe | 7.43 | 6.34 [30] |
| Cs | 3.32 | 3.79 [30] |
| Ba | 3.13 | 2.43 [30] |
| Lu | 3.55 | |
| Hf | 3.46 | 3.95 [32] |
| Ta | 3.98 | 3.75 [30] |
| W | 4.26 | 4.32 [30] |
| Re | 4.57 | 5.41 [32] |
| Os | 5.00 | 4.5 [35] |
| Ir | 5.23 | 4.83 [32] |
| Pt | 5.45 | 5.18 [32] |
| Au | 6.07 | 6.4 [30] |
| Hg | 8.72 | |
| Tl | 5.55 | 5.8 [36] |
| Pb | 5.11 | 5.335 [30] |
| Bi | 7.64 | 2.4 [30] |
| Po | 5.35 | |
| Rn | 8.57 | |

**Tab. 2.5** Elastic constants (in GPa) by means of VASP-PW91 and from experiment (both taken from [37])

| | $C_{11,VASP}$ | $C_{11,exp}$ | $C_{12,VASP}$ | $C_{12,exp}$ | $C_{33,VASP}$ | $C_{33,exp}$ |
|---|---|---|---|---|---|---|
| Li | 14.6 | 14.8 | 13.8 | 12.5 | 14.6 | 14.8 |
| Be | 312.2 | 299.4 | 24.6 | 27.6 | 377.9 | 342.2 |
| Na | 9.8 | 9.45 | 7.9 | 7.79 | 9.8 | 9.45 |
| Mg | 58.1 | 63.48 | 27.6 | 25.94 | 64.7 | 66.45 |
| Al | 101.0 | 114.3 | 61.0 | 61.92 | 101.0 | 114.3 |
| K | 3.7 | 4.16 | 3.2 | 3.41 | 3.7 | 4.16 |
| Ca | 22.1 | 22.8 | 15.3 | 16 | 22.1 | 22.8 |
| Sc | 104.8 | 99.3 | 37.7 | 39.7 | 105.2 | 107 |
| Ti | 174.8 | 176.1 | 87.5 | 86.9 | 189.5 | 190.5 |
| V | 272.0 | 232.4 | 144.8 | 119.36 | 272.0 | 232.4 |
| Cr | 247.6 | 391 | 73.4 | 89.6 | 247.6 | 391 |
| Fe | 279.2 | 243.1 | 148.8 | 138.1 | 279.2 | 243.1 |
| Co | 363.4 | 319.5 | 168.2 | 166.1 | 411.7 | 373.6 |
| Ni | 275.5 | 261.2 | 160.1 | 150.8 | 275.5 | 261.2 |
| Cu | 174.8 | 176.2 | 122.8 | 124.94 | 174.8 | 176.2 |
| Zn | 159.5 | 179.09 | 56.0 | 37.5 | 57.0 | 68.8 |
| Rb | 3.1 | 3.42 | 2.7 | 2.88 | 3.1 | 3.42 |
| Sr | 15.0 | 15.3 | 10.5 | 10.3 | 15.0 | 15.3 |
| Y | 78.0 | 83.4 | 24.8 | 29.1 | 82.4 | 80.1 |
| Zr | 145.3 | 155.4 | 67.3 | 67.2 | 166.1 | 172.5 |
| Nb | 247.2 | 252.7 | 140.0 | 133.2 | 247.2 | 252.7 |
| Mo | 466.0 | 450.02 | 165.2 | 172.92 | 466.0 | 450.02 |
| Tc | 491.4 | 433 | 222.4 | 199 | 546.8 | 470 |
| Ru | 558.9 | 576.3 | 188.5 | 187.2 | 631.8 | 640.5 |
| Rh | 405.3 | 413 | 185.5 | 194 | 405.3 | 413 |
| Pd | 198.0 | 234.12 | 155.7 | 176.14 | 198.0 | 234.12 |
| Ag | 115.9 | 131.44 | 85.1 | 97.3 | 115.9 | 131.44 |
| Cd | 93.2 | 129.23 | 40.7 | 39.99 | 43.9 | 56.68 |
| Cs | 2.1 | 2.59 | 2.0 | 2.17 | 2.1 | 2.59 |
| Ba | 12.3 | 12.6 [38,39] | 7.6 | 11.1 [38,39] | 12.3 | 12.6 [38,39] |
| Hf | 183.6 | 190.1 | 71.1 | 74.5 | 197.9 | 204.4 |
| Ta | 260.9 | 266.32 | 165.2 | 158.16 | 260.9 | 266.32 |
| W | 517.8 | 532.55 | 201.7 | 204.95 | 517.8 | 532.55 |
| Re | 613.1 | 644.6 | 279.9 | 277 | 674.5 | 717 |
| Os | 729.6 | 763.3 | 230.0 | 227.9 | 816.9 | 843.2 |
| Ir | 580.8 | 599.47 | 232.0 | 255.82 | 580.8 | 599.47 |
| Pt | 296.4 | 358 | 225.6 | 253.6 | 296.4 | 358 |
| Au | 159.1 | 201.63 | 136.7 | 169.67 | 159.1 | 201.63 |
| Tl | 34.9 | 44.4 | 29.2 | 37.6 | 48.7 | 60.2 |
| Pb | 75.2 | 55.54 | 60.2 | 45.42 | 75.2 | 55.54 |

| | $C_{13,VASP}$ | $C_{13,exp}$ | $C_{44,VASP}$ | $C_{44,exp}$ |
|---|---|---|---|---|
| Li | 13.8 | 12.5 | 11.5 | 10.8 |
| Be | 10.9 | 11 | 165.4 | 166.2 |
| Na | 7.9 | 7.79 | 6.6 | 6.18 |
| Mg | 21.6 | 21.7 | 14.2 | 18.42 |
| Al | 61 | 61.92 | 25.4 | 31.62 |
| K | 3.2 | 3.41 | 2.6 | 2.86 |
| Ca | 15.3 | 16 | 13.2 | 14 |
| Sc | 29.3 | 29.4 | 31.6 | 27.7 |
| Ti | 80 | 68.3 | 40.9 | 50.8 |
| V | 144.8 | 119.36 | 17.6 | 45.95 |
| Cr | 73.4 | 89.6 | 48.3 | 103.2 |
| Fe | 148.8 | 138.1 | 93 | 121.9 |
| Co | 116.3 | 102.1 | 91.3 | 82.4 |
| Ni | 160.1 | 150.8 | 126.3 | 131.7 |
| Cu | 122.8 | 124.94 | 76.3 | 81.77 |
| Zn | 51.8 | 55.4 | 23.2 | 45.95 |
| Rb | 2.7 | 2.88 | 2 | 2.21 |
| Sr | 10.5 | 10.3 | 13.9 | 9.9 |
| Y | 22.7 | 19 | 26.4 | 26.9 |
| Zr | 69.5 | 64.6 | 24.3 | 36.3 |
| Nb | 140 | 133.2 | 14.2 | 30.97 |
| Mo | 165.2 | 172.92 | 99.5 | 125.03 |
| Tc | 183.4 | 199 | 129.9 | 177 |
| Ru | 176.4 | 167.3 | 179.9 | 189.1 |
| Rh | 185.5 | 194 | 176.5 | 184 |
| Pd | 155.7 | 176.14 | 69.7 | 71.17 |
| Ag | 85.1 | 97.3 | 42.1 | 51.08 |
| Cd | 34.5 | 40.95 | 11.8 | 24.2 |
| Cs | 2 | 2.17 | 1.4 | 1.6 |
| Ba | 7.6 | 11.1 [38,39] | 10.5 | 9.5 [38,39] |
| Hf | 71.1 | 65.5 | 51.1 | 60 |
| Ta | 165.2 | 158.16 | 70.4 | 87.36 |
| W | 201.7 | 204.95 | 139.4 | 163.13 |
| Re | 223 | 195.9 | 142.5 | 168.5 |
| Os | 229 | 218 | 251.5 | 269.3 |
| Ir | 232 | 255.82 | 249.8 | 268.82 |
| Pt | 225.6 | 253.6 | 50.7 | 77.4 |
| Au | 136.7 | 169.67 | 27.6 | 45.44 |
| Tl | 24.8 | 30 | 4.7 | 8.8 |
| Pb | 60.2 | 45.42 | 25.8 | 19.42 |

# 3. Difference between codes

For each element the crystal structure is the one defined by the corresponding CIF file in CIFs.tar.gz.

**Tab. 3.1** Equilibrium volume $V_0$ (in Å$^3$/atom), bulk modulus $B_0$ (in GPa) and its pressure derivative $B_1$ (dimensionless) by means of WIEN2k-PBE for fixed geometries. These data are available in WIEN2k.txt as well, as an unformatted text file

| | $V_{0,WIEN2k}$ | $B_{0,WIEN2k}$ | $B_{1,WIEN2k}$ |
|---|---|---|---|
| H | 17.39 | 10.3 | 3.03 |
| He | 17.78 | 0.8 | 6.53 |
| Li | 20.22 | 13.9 | 3.75 |
| Be | 7.92 | 123.0 | 3.15 |
| B | 7.25 | 237.6 | 3.48 |
| C | 11.65 | 209.6 | 3.57 |
| N | 28.90 | 54.3 | 3.75 |
| O | 18.56 | 51.2 | 3.93 |
| F | 19.35 | 35.0 | 4.25 |
| Ne | 24.35 | 1.2 | 8.66 |
| Na | 37.09 | 7.7 | 3.74 |
| Mg | 22.93 | 35.7 | 4.26 |
| Al | 16.50 | 77.5 | 4.67 |
| Si | 20.55 | 88.7 | 4.23 |
| P | 21.61 | 68.9 | 4.42 |
| S | 17.35 | 85.5 | 4.44 |
| Cl | 39.18 | 19.3 | 4.49 |
| Ar | 52.21 | 0.7 | 7.84 |
| K | 73.71 | 3.6 | 3.73 |
| Ca | 42.21 | 17.3 | 3.17 |
| Sc | 24.62 | 54.6 | 3.40 |
| Ti | 17.41 | 112.7 | 3.59 |
| V | 13.52 | 185.2 | 3.73 |
| Cr | 11.91 | 183.8 | 7.37 |
| Mn | 11.61 | 131.2 | 0.85 |
| Fe | 11.45 | 196.1 | 6.14 |
| Co | 10.95 | 216.2 | 5.08 |
| Ni | 10.99 | 204.7 | 4.85 |
| Cu | 12.02 | 143.7 | 5.20 |
| Zn | 15.27 | 75.6 | 5.38 |
| Ga | 20.38 | 49.1 | 5.33 |
| Ge | 24.09 | 59.5 | 5.08 |
| As | 22.57 | 69.7 | 4.29 |
| Se | 29.97 | 47.6 | 4.55 |
| Br | 39.78 | 22.6 | 5.15 |
| Kr | 65.23 | 0.9 | 22.01 |
| Rb | 91.13 | 2.8 | 2.32 |
| Sr | 54.56 | 11.3 | 4.17 |
| Y | 32.86 | 41.3 | 2.95 |

| | | | |
|---|---|---|---|
| Zr | 23.40 | 94.1 | 3.25 |
| Nb | 18.16 | 168.7 | 3.50 |
| Mo | 15.83 | 260.4 | 4.26 |
| Tc | 14.47 | 301.4 | 4.56 |
| Ru | 13.81 | 315.4 | 4.96 |
| Rh | 14.08 | 260.6 | 5.44 |
| Pd | 15.33 | 170.4 | 5.85 |
| Ag | 17.86 | 91.3 | 5.80 |
| Cd | 22.87 | 44.2 | 7.09 |
| In | 27.50 | 34.8 | 4.87 |
| Sn | 36.88 | 36.0 | 5.04 |
| Sb | 31.79 | 50.7 | 4.50 |
| Te | 35.01 | 44.8 | 4.70 |
| I | 50.34 | 18.7 | 5.22 |
| Xe | 87.32 | 0.6 | -0.72 |
| Cs | 117.75 | 2.0 | 3.59 |
| Ba | 63.20 | 8.4 | 3.30 |
| Lu | 29.06 | 47.7 | 4.05 |
| Hf | 22.55 | 108.1 | 3.23 |
| Ta | 18.30 | 193.7 | 4.77 |
| W | 16.17 | 302.6 | 4.30 |
| Re | 14.99 | 364.6 | 4.47 |
| Os | 14.32 | 402.2 | 4.35 |
| Ir | 14.53 | 341.7 | 6.96 |
| Pt | 15.68 | 251.8 | 5.34 |
| Au | 17.99 | 139.9 | 5.99 |
| Hg | 29.72 | 8.2 | 8.08 |
| Tl | 31.46 | 26.7 | 4.57 |
| Pb | 32.00 | 39.6 | 5.95 |
| Bi | 36.94 | 42.6 | 4.63 |
| Po | 37.57 | 45.5 | 5.02 |
| Rn | 92.76 | 0.5 | 13.13 |

**Tab. 3.2** Equilibrium volume $V_0$ (in Å$^3$/atom), bulk modulus $B_0$ (in GPa) and its pressure derivative $B_1$ (dimensionless) by means of VASP-PBE and GPAW-PBE for fixed geometries

| | $V_{0,VASP}$ | $B_{0,VASP}$ | $B_{1,VASP}$ | $V_{0,GPAW}$ | $B_{0,GPAW}$ | $B_{1,GPAW}$ |
|---|---|---|---|---|---|---|
| H | 17.44 | 10.1 | 3.03 | 17.46 | 10.3 | 2.93 |
| He | 17.72 | 0.9 | 7.42 | 17.69 | 0.8 | 6.73 |
| Li | 20.29 | 13.8 | 3.16 | 20.28 | 14.0 | 3.41 |
| Be | 7.92 | 123.3 | 3.29 | 8.01 | 123.3 | 3.37 |
| B | 7.25 | 237.0 | 3.47 | 7.24 | 237.1 | 3.53 |
| C | 11.66 | 208.4 | 3.56 | 11.65 | 208.7 | 3.62 |
| N | 29.65 | 56.4 | 3.86 | 28.91 | 54.0 | 3.67 |
| O | 19.19 | 51.4 | 4.06 | 19.28 | 53.6 | 3.96 |
| F | 19.54 | 34.2 | 4.20 | 19.21 | 33.7 | 4.50 |
| Ne | 24.61 | 1.1 | 14.48 | 23.75 | 2.1 | 20.67 |
| Na | 37.07 | 7.7 | 3.04 | 37.04 | 7.8 | 3.91 |
| Mg | 22.85 | 36.5 | 3.92 | 22.97 | 36.3 | 4.18 |
| Al | 16.49 | 77.3 | 4.65 | 16.51 | 78.2 | 4.61 |
| Si | 20.45 | 88.8 | 4.30 | 20.52 | 88.8 | 4.36 |
| P | 21.36 | 68.5 | 4.34 | 21.53 | 68.1 | 4.44 |
| S | 17.17 | 83.5 | 4.14 | 17.22 | 83.7 | 4.32 |
| Cl | 38.21 | 19.2 | 4.33 | 38.95 | 19.0 | 4.59 |
| Ar | 52.65 | 0.8 | 7.35 | 52.66 | 0.8 | 3.27 |
| K | 73.84 | 3.6 | 3.82 | 73.78 | 3.6 | 2.49 |
| Ca | 42.17 | 17.5 | 3.02 | 42.46 | 17.4 | 3.19 |
| Sc | 24.66 | 54.4 | 3.41 | 24.66 | 54.2 | 3.10 |
| Ti | 17.37 | 112.5 | 3.60 | 17.26 | 114.4 | 3.71 |
| V | 13.48 | 181.6 | 4.02 | 13.73 | 185.5 | 4.38 |
| Cr | 11.83 | 176.8 | 7.17 | 11.87 | 161.8 | 6.67 |
| Mn | 11.57 | 115.4 | 0.35 | 11.75 | 126.6 | 1.12 |
| Fe | 11.38 | 185.7 | 4.91 | 11.48 | 196.7 | 5.03 |
| Co | 10.88 | 210.8 | 4.99 | 10.92 | 212.4 | 5.00 |
| Ni | 10.94 | 193.7 | 4.92 | 10.92 | 203.6 | 4.60 |
| Cu | 12.03 | 136.8 | 5.10 | 12.10 | 139.4 | 4.59 |
| Zn | 15.29 | 74.2 | 5.62 | 15.25 | 75.1 | 4.80 |
| Ga | 20.36 | 48.9 | 5.09 | 20.52 | 50.3 | 5.24 |
| Ge | 23.91 | 58.8 | 4.78 | 23.98 | 60.1 | 4.84 |
| As | 22.69 | 68.7 | 4.29 | 22.64 | 68.9 | 4.43 |
| Se | 29.83 | 47.2 | 4.48 | 29.75 | 47.2 | 4.61 |
| Br | 39.47 | 22.5 | 4.85 | 40.38 | 20.8 | 4.66 |
| Kr | 66.56 | 0.7 | 4.82 | 65.58 | 0.8 | 13.16 |
| Rb | 91.24 | 2.8 | 3.73 | 91.17 | 2.7 | 3.06 |
| Sr | 54.54 | 11.1 | 4.59 | 55.15 | 11.2 | 3.68 |
| Y | 32.92 | 41.4 | 3.20 | | | |
| Zr | 23.53 | 93.8 | 3.58 | 23.46 | 94.9 | 3.38 |
| Nb | 18.34 | 171.8 | 3.97 | 18.23 | 174.2 | 3.78 |
| Mo | 15.92 | 262.9 | 4.34 | 15.89 | 263.7 | 4.38 |
| Tc | 14.60 | 298.5 | 4.55 | | | |
| Ru | 13.84 | 311.5 | 4.95 | 14.09 | 310.9 | 4.87 |
| Rh | 14.18 | 254.2 | 5.25 | 14.32 | 255.2 | 5.42 |

| | | | | | | |
|---|---|---|---|---|---|---|
| Pd | 15.44 | 168.2 | 5.64 | 15.41 | 167.3 | 5.98 |
| Ag | 18.05 | 89.1 | 5.78 | 18.07 | 90.7 | 5.52 |
| Cd | 23.01 | 43.8 | 7.23 | 22.87 | 43.3 | 6.28 |
| In | 27.54 | 35.4 | 5.34 | 27.53 | 35.1 | 5.60 |
| Sn | 36.86 | 35.8 | 4.85 | 36.90 | 36.0 | 4.90 |
| Sb | 31.79 | 50.9 | 4.54 | | | |
| Te | 34.96 | 45.0 | 4.72 | 34.17 | 46.1 | 4.81 |
| I | 50.12 | 18.7 | 5.09 | 51.15 | 17.6 | 4.88 |
| Xe | 87.77 | 0.5 | 7.76 | | | |
| Cs | 116.96 | 2.0 | 3.48 | 117.01 | 2.1 | 3.59 |
| Ba | 63.55 | 8.9 | 3.11 | 63.51 | 8.9 | 2.95 |
| Lu | 29.47 | 47.2 | 3.44 | | | |
| Hf | 22.50 | 107.8 | 3.48 | | | |
| Ta | 18.33 | 194.3 | 3.97 | 18.52 | 198.4 | 3.99 |
| W | 16.23 | 304.4 | 4.30 | 16.44 | 307.5 | 4.35 |
| Re | 14.93 | 372.5 | 4.55 | | | |
| Os | 14.36 | 400.9 | 4.95 | 14.52 | 397.9 | 4.98 |
| Ir | 14.57 | 346.0 | 5.17 | 14.70 | 351.6 | 5.39 |
| Pt | 15.72 | 248.1 | 5.53 | 15.79 | 247.6 | 5.67 |
| Au | 18.18 | 136.4 | 5.91 | 18.21 | 137.8 | 5.77 |
| Hg | 29.94 | 7.6 | 12.94 | | | |
| Tl | 31.52 | 26.5 | 5.43 | | | |
| Pb | 32.08 | 39.8 | 4.40 | 32.10 | 39.1 | 5.56 |
| Bi | 36.99 | 42.5 | 4.55 | 36.97 | 42.9 | 4.76 |
| Po | 37.53 | 45.4 | 4.63 | | | |
| Rn | 93.11 | 0.6 | 7.24 | | | |

[1] C. Kittel, *Introduction to Solid State Physics* , 8th ed. (John Wiley & Sons, Inc, 2005).
[2] N. Greenwood and A. Earnshaw, *Chemistry of the Elements* , 2nd ed. (Butterworth-Heinemann, 1997).
[3] T. Tohei, A. Kuwabara, F. Oba, and I. Tanaka, Phys. Rev. B **73**, 064304 (2006).
[4] V. Moruzzi, J. Janak, and K. Schwarz, Phys. Rev. B **37**, 790 (1988).
[5] P. Villars and J. Daams, J. Alloys Compd. **197**, 177 (1993).
[6] L. Bolz, M. Boyd, F. Mauer, and H. Peiser, Acta Crystallogr. **12**, 247 (1959).
[7] L. Meyer, C. Barrett, and S. Greer, J. Chem. Phys. **49**, 1902 (1968).
[8] D. Batchelder, D. Losee, and R. Simmons, Phys. Rev. **162**, 767 (1967).
[9] B. Powell, K. Heal, and B. Torrie, Mol. Phys. **53**, 929 (1984).
[10] O. Peterson, D. Batchelder, and R. Simmons, Phys. Rev. **150**, 703 (1966).
[11] D. Losee and R. Simmons, Phys. Rev. **172**, 944 (1968).
[12] D. Sears and H. Klug, J. Chem. Phys. **37**, 3002 (1962).
[13] C. Swenson, Phys. Rev. **111**, 82 (1958).
[14] D. Lide (ed.), *CRC Handbook of Chemistry and Physics* , 89th ed. (CRC Press, Boca Raton, Florida, 2008-2009).
[15] J. Nelson and D. Riley, Proc. Phys. Soc. London **57**, 477 (1945).
[16] R. Keyes, Phys. Rev. **92**, 580 (1953).
[17] J. Wallis, I. Sigalas, and S. Hart, J. Appl. Crystallogr. **19**, 273 (1986).
[18] R. Pawar and V. Deshpande, J. Mater. Sci. **5**, 1061 (1970).
[19] M. Anderson and C. Swenson, Phys. Rev. B **28**, 5395 (1983).
[20] Y. Tsuru, Y. Shinzato, Y. Saito, M. Shimazu, M. Shiono, and M. Morinaga, J. Ceram. Soc. Jpn. **118**, 241 (2010).
[21] E. Kim and C. Chen, Phys. Lett. A **326**, 442 (2004).
[22] T. Scott, Phys. Rep. **27C**, 89 (1976).
[23] Y. Endoh, G. Shirane, and J. Skalyo, Phys. Rev. B **11**, 1681 (1975).
[24] E.-F. Düsing, W. Grosshans, and W. Holzapfel, J. Phys. Colloques (Paris) **45**, 203 (1984).
[25] G. Keeler and D. Batchelder, J. Phys. C **3**, 510 (1970).
[26] H. Fujihisa and K. Takemura, Phys. Rev. B **52**, 13257 (1995).
[27] J. Skalyo, Y. Endoh, and G. Shirane, Phys. Rev. B **9**, 1797 (1974).
[28] D. Price, J. Rowe, and R. Nicklow, Phys. Rev. B **3**, 1268 (1971).
[29] N. Lurie, G. Shirane, and J. Skalyo, Phys. Rev. B **9**, 2661 (1974).
[30] E. Knittle, in *Mineral Physics and Crystallography: A Handbook of Physical Constants* , edited by T. Ahrens (American Geophysical Union Press, 1995) pp. 98-142.
[31] S. Batsanov, in *Effects of Explosions on Materials: Modification and Synthesis under High Pressure Shock Compression* (Springer, New York, 1994).
[32] M. Guinan and D. Steinberg, J. Phys. Chem. Solids **35**, 1501 (1974).
[33] C. Menoni, J. Hu, and I. Spain, Phys. Rev. B **34**, 362 (1986).
[34] H. Beister, K. Strössner, and K. Syassen, Phys. Rev. B **41**, 5535 (1990).
[35] T. Kenichi, Phys. Rev. B **70**, 012101 (2004).
[36] J. Li, S. Liang, H. Guo and B. Liu, J. Alloys Compd. **431**, 23 (2007).
[37] S. Shang, A. Saengdeejing, Z. Mei, D. Kim, H. Zhang, S. Ganeshan, Y. Wang, and Z. Liu, Comput. Mater. Sci. **48**, 813 (2010).
[38] L. Hector, J. Herbst, W. Wolf, P. Saxe, and G. Kresse, Phys. Rev. B **76**, 014121 (2007).
[39] U. Buchenau, M. Heiroth, H. Schober, J. Evers, and G. Oehlinger, Phys. Rev. B **30**, 3502 (1984).
